# Supplementary material for: Making Decisions under Outcome Performativity
Source: arXiv:2210.01745 source file (2023-01-07)
Supplement: Supplementary file 1 [file appendix.tex]

\newpage
--------------------- FOR SAFE KEEPING

identifies two solution concepts for performative prediction problems: \emph{optimality} and \emph{stability}.
A decision rule  is performative optimal if $h_\mathrm{po}$ achieves the best possible performance on the induced distribution.
Formally, for hypothesis class $\Hcal$ and loss function $\ell$, performative optimality is defined by the following global optimization over $\Hcal$:

where $\D(h)$ is the distribution over $(x,y)$ pairs induced by predictions according to hypothesis $h$.

% \mpk{optimality is a very strong notion.}
While syntactically similar to the standard learning objective, performative optimality seems to be a significantly harder task than supervised learning, computationally and information-theoretically.
Standard arguments from supervised learning (e.g.,\ uniform convergence to establish bounded sample complexity) fail spectacularly in the performative setting because the distribution of examples may depend on the chosen hypothesis.
To date, the only known methods for obtaining performative optimality efficiently require strong distributional assumptions.
For instance, \cite{miller2021outside} give learning algorithms for performative optimal predictors, assuming that the process of generating outcomes for individuals and the mechanism of performativity are governed by explicit, simple (linear) models.

A concrete challenge for learning algorithms working in the performative setting is that optimal hypotheses may appear locally suboptimal; that is, $h_\mathrm{po}$ may not be a loss minimizer under $\D(h_\mathrm{po})$.
\begin{gather*}
h_\mathrm{po} \not \in \argmin_{h \in \Hcal}\E_{\D(h_\mathrm{po})}[\ell(h(x),y)]
\end{gather*}
In contrast, predictors satisfying this notion of local optimality, which \cite{performative} calls performative stable, are best understood as a ``stationary'' decision rules.
The main results of \cite{performative} characterizes performative stability as the set of predictors achieved through iterative retraining.
Further, \cite{performative} shows that the loss achieved by performative stable points can be \emph{arbitrarily worse} than the performative optimal.
Unlike performative stability, performative optimality is not obviously achieved by any simple method like iterative retraining.
This separation has seeded pessimism about performative optimality.
Without contrived simplifying assumptions, learning performative optimal predictors remains an infeasible problem.

------------ MPK outline for our contributions --------

\paragraph{Universal Adaptability.}

    \begin{itemize}
        \item The paradigm of learning an outcome probability function $\pt$ and post-processing is very powerful.  But, inherently, it treats individuals as units.  That is, it can't handle input performativity.
        \item We show that we can get the next best thing.
        \item adapting a guarantee recently studied in statistical inference problems, we show how to obtain \emph{universally adaptable} omnipredictors.
        \item Intuitively, UA performative omnipredictors $\pt$ give the omnipredictor guarantee, not just on the original distribution over individuals, but on a rich class of potential distribution shifts.
        Shifts are specified by a class of importance weights $\cW$, where $\D_\omega$ is reweighted by some $\omega \in \cW$.
        \item \textbf{THEOREM:}  For any $\cW$, there exist $(\cL,\Hcal,\eps)$-omnipredictors that are $\cW$-universally adaptable with complexity \mpk{add in complexity of $\cW$}.
    \end{itemize}

\paragraph{Learning Performative Omnipredictors.}
    
    \begin{itemize}
        \item The existence theorems are consequences of a generic learning pardigm.
        \item We show that it's possible to instantiate the paradigm using RCT data.
        \item \textbf{THEOREM:}  There exists a learning algorithm for $(\cL,\Hcal,\eps)$-performative omnipredictors that uses:
        \begin{itemize}
            \item $m \le \card{\cL}  \cdot \card{\Ych} \cdot \mathrm{VC}(\Hcal) \cdot \poly(1/\eps)$ RCT samples \mpk{is VC really the right notion?  if we have $\card{\Ych}$ then should we have another measure of complexity?  I guess $\log\card{\Hcal}$ isn't the worst for now.}
            \item $\card{\cL} \cdot \poly(1/\eps)$ calls to an agnostic learner for $\Hcal$.
        \end{itemize}
    \end{itemize}

--------------- MPK outline for technical overview ---------

\newpage

Original work on omniprediction: multicalibration implies omniprediction
\begin{itemize}
    \item obtain strong results in the supervised learning setting
    \item as we discuss in Section~\ref{sec:calibration}, calibration is possible, but can be inefficient in the performative world (even without multi)
    \item we turn to the abstraction of outcome indistinguishability \cite{oi}
\end{itemize}

Main tool:  performative outcome indistinguishability.
\begin{itemize}
    \item In the supervised world, there is a tight correspondence between OI and multicalibration.  Thus, off-the-bat, some instantiation of OI implies omniprediction.
    \item But OI gives a very nice interface to work with in the performative setting
    \item We require that our predictor $\pt$ generates outcomes that are indistinguishable from those generated by $\ps$
    \item But under which decision rules?
    \item Omniprediction constraints give us guidance:  the hypotheses we wish to compete against
\end{itemize}

\begin{definition}[Performative OI]
def
\end{definition}

Post-processing:
\begin{itemize}
    \item Omnipredictor $\pt$ has to be good under post-processing
    \item Require OI to hold even under the optimal decision rules according to $\ell$
\end{itemize}

\begin{definition}[Performative Decision OI]
def
\end{definition}

Once we have the right abstractions in place, the proof of omniprediction is immediate!
\begin{itemize}
    \item loss of $h(x)$ same under $\ys \sim \ps(x,h(x))$ and $\yt \sim \pt(x,h(x))$
    \item $\ft_\ell(x)$ is the loss minimizer $\yt \sim \pt(x,\ft_\ell(x))$, so in particular, better than $h(x)$
    \item loss of $\ft_\ell(x)$ same under $\yt \sim \pt(x,\ft_\ell(x))$ and $\ys \sim \ps(x,\ft_\ell(x))$
    \item Thus, loss of $h(x)$ is at least that of $\ft_\ell(x)$ on true outcomes.
\end{itemize}
This direct proof strategy is inspired by a concurrent work on omniprediction in the supervised setting \cite{gopalan2022personal}.

Given our approach is based on OI, we can appeal to many of the existing tools from the OI / multicalibration literature.
\begin{itemize}
    \item universal adaptability:  natural consequence.  need to be careful, though, to only touch the distribution over $\Xcal$.  Need to be able to anticipate the possible shifts, while maintaining the optimal decision rule on each individual.
    \item general reduction from learning to auditing works!
\end{itemize}

Learning:
\begin{itemize}
    \item How do we implement the auditor?
    \item Observation:  RCT-style data suffices!  In particular, given RCT data we can reduce the problem to \emph{supervised learning} primitives.
    \item highlights the power of free experimentation:  if we can experiment for a while to collect data, then we can reduce this performative problem to a non-performative problem.
\end{itemize}

Finally, we look into notions of multicalibration in the performative setting
\begin{itemize}
    \item calibration is a bit of a non-starter
    \item in particular, the complexity of calibration scales exponentially in the number of \emph{decisions}, not just the number of outcomes!  this is a significant difference from supervised learning
    \item highlights the importance of having the OI framework:  can design distinguishers exactly for the task at hand.
    \item on the flip side, we show that a variant of multiaccuracy suffices to obtain performative OI for all losses
    \item only requirement then, is to obtain decision OI efficiently.  this too can be achieved for all losses simultaneously, via decision calibration.
\end{itemize}

\paragraph{Notation}
\begin{itemize}
	\item Individual features (units for prediction) $x \in \cX$, where $\cX$ assumed discrete
	\item Predictions (actions or decision) $\yhat \in \cYh$, assumed discrete. We let $k \defeq |\cYh|$
	\item We use $\Delta(\calX)$ to denote the simplex  or set of distributions over a discrete set $\cX$. 
	\item Outcomes $y \in \cY$, assumed discrete 	\item Nature's conditional distribution $\ps : \cX \times \cYh \rightarrow \Delta(\cY)$
	\item Learner's model of nature $\pt: \cX \times \cYh \rightarrow \Delta(\cY)$
	\item Loss functions $\ell: \cX \times \cYh \times \cY \rightarrow \R_{\geq 0}$  and set of losses $\cL \subseteq \cX \times \cYh \times \cY \rightarrow \R_{\geq 0}$ 
	\item Importance weights $\omega: \cX \rightarrow \R_{\geq 0}$, set of importance weights $\cW \subseteq \cX \rightarrow \R_{\geq 0}$.
	\item $\cD$ is a distribution over covariate $\cX$, $\Sd \subseteq \Delta(\cX)$ is a set of distributions over $\cX$
	\item For a set of functions $\cF: \cZ \rightarrow \R_{\geq 0}$, $\|\cF\|_{\infty} = \sup_{z \in \cZ, f \in \cF} f(z)$. We use the shorthand, $\lmax  =\|\cL \|_{\infty}$ and $\omax = \|\cW\|_{\infty}$.
	\item The Euclidean projection onto the simplex: $\Pi$
	\item For a fixed $\ell \in \cL$, we define $f_{\ell,p}: \cX \to \cYh$ to be the optimal post-processing of $p$ according to $\ell$. 
More specifically, for every $x \in \cX$,
\begin{align*}
    f_{\ell,p}(x) = \argmin_{\yhat \in \cYh} \E_{\yt \sim p(x,\yhat)}[\ell(x, \yhat,\yt)].
\end{align*}
Note that $f_{\ell, p}$ is defined pointwise, without regard to the marginal distribution over $\cX$. Some shorthand,
\begin{align*}
	\ft_\ell \defeq f_{\ell, \pt}, \quad f_{\ell, t} = f_{\ell,p^{(t)}}
\end{align*}
\end{itemize}

\clearpage
